# Supplementary material for: Automatic Routing of Goldstone Diagrams using Genetic Algorithms
Source: arXiv:1907.00426 ancillary file (2019-06-30)
Supplement: Supplementary file 1 [file Supporting_Information.pdf]

# 1 Projected (Similarity Transformed) Coupled Cluster

Table 1: Optimized CCSD Goldstone diagrams for energy, singles and doubles projection of the similarity transformed CC ansatz for  $\hat{H}_N = \hat{F}_N + \hat{V}_N$ . To identify specific diagrams, each has been assigned to a unique index. Furthermore, the needed generations (iterations) of the genetic algorithm to convergence and the final costs (with an accuracy of  $10^{-2}$ ) of the diagram are shown.

| Index | Projection           | Contraction                                               | Diagram | Generations | Cost   |
|-------|----------------------|-----------------------------------------------------------|---------|-------------|--------|
| 0     | $\langle \Psi_0  $   | $\overline{\hat{F}_N \hat{T}_1} \Psi_0 \rangle$           |         | 212         | -10.00 |
| 1     | $\langle \Psi_0  $   | $\overline{\hat{V}_N \hat{T}_1 \hat{T}_1} \Psi_0 \rangle$ |         | 514         | -21.00 |
| 2     | $\langle \Psi_0  $   | $\overline{\hat{V}_N \hat{T}_2} \Psi_0 \rangle$           |         | 522         | -21.00 |
| 3     | $\langle \Psi_I^A  $ | $\hat{F}_N \Psi_0 \rangle$                                |         | 313         | 0.00   |
| 4     | $\langle \Psi_I^A  $ | $\overline{\hat{F}_N \hat{T}_1} \Psi_0 \rangle$           |         | 798         | 0.00   |
| 5     | $\langle \Psi_I^A  $ | $\overline{\hat{F}_N \hat{T}_1} \Psi_0 \rangle$           |         | 787         | 0.00   |
| 6     | $\langle \Psi_I^A  $ | $\overline{\hat{F}_N \hat{T}_1 \hat{T}_1} \Psi_0 \rangle$ |         | 1000        | 1.63   |
| 7     | $\langle \Psi_I^A  $ | $\overline{\hat{F}_N \hat{T}_2} \Psi_0 \rangle$           |         | 1099        | -10.00 |
| 8     | $\langle \Psi_I^A  $ | $\overline{\hat{V}_N \hat{T}_1 \hat{T}_2} \Psi_0 \rangle$ |         | 1807        | -7.71  |
| 9     | $\langle \Psi_I^A  $ | $\overline{\hat{V}_N \hat{T}_1 \hat{T}_1} \Psi_0 \rangle$ |         | 1231        | -10.00 |
| 10    | $\langle \Psi_I^A  $ | $\overline{\hat{V}_N \hat{T}_1 \hat{T}_2} \Psi_0 \rangle$ |         | 1996        | -7.71  |
| 11    | $\langle \Psi_I^A  $ | $\overline{\hat{V}_N \hat{T}_1 \hat{T}_2} \Psi_0 \rangle$ |         | 1894        | -20.00 |
| 12    | $\langle \Psi_I^A  $ | $\overline{\hat{V}_N \hat{T}_2} \Psi_0 \rangle$           |         | 1508        | -9.34  |
| 13    | $\langle \Psi_I^A  $ | $\overline{\hat{V}_N \hat{T}_1 \hat{T}_1} \Psi_0 \rangle$ |         | 1142        | -10.00 |

|    |                            |                                                          |  |      |        |
|----|----------------------------|----------------------------------------------------------|--|------|--------|
| 14 | $\langle \Psi_I^A  $       | $\hat{V}_N \hat{T}_1 \Psi_0 \rangle$                     |  | 782  | -10.00 |
| 15 | $\langle \Psi_I^A  $       | $\hat{V}_N \hat{T}_2 \Psi_0 \rangle$                     |  | 1641 | -9.34  |
| 16 | $\langle \Psi_I^A  $       | $\hat{V}_N \hat{T}_1 \hat{T}_1 \hat{T}_1 \Psi_0 \rangle$ |  | 1608 | -8.37  |
| 17 | $\langle \Psi_{IJ}^{AB}  $ | $\hat{V}_N \hat{T}_1 \Psi_0 \rangle$                     |  | 1352 | 0.00   |
| 18 | $\langle \Psi_{IJ}^{AB}  $ | $\hat{V}_N \hat{T}_1 \hat{T}_2 \Psi_0 \rangle$           |  | 2707 | 1.92   |
| 19 | $\langle \Psi_{IJ}^{AB}  $ | $\hat{V}_N \hat{T}_2 \Psi_0 \rangle$                     |  | 2281 | -10.00 |
| 20 | $\langle \Psi_{IJ}^{AB}  $ | $\hat{V}_N \hat{T}_1 \hat{T}_2 \Psi_0 \rangle$           |  | 2900 | -10.00 |
| 21 | $\langle \Psi_{IJ}^{AB}  $ | $\hat{V}_N \hat{T}_1 \hat{T}_2 \Psi_0 \rangle$           |  | 2923 | -10.00 |
| 22 | $\langle \Psi_{IJ}^{AB}  $ | $\hat{V}_N \hat{T}_1 \hat{T}_1 \Psi_0 \rangle$           |  | 2198 | -1.00  |
| 23 | $\langle \Psi_{IJ}^{AB}  $ | $\hat{V}_N \hat{T}_1 \hat{T}_1 \hat{T}_1 \Psi_0 \rangle$ |  | 2410 | 1.92   |
| 24 | $\langle \Psi_{IJ}^{AB}  $ | $\hat{V}_N \hat{T}_1 \Psi_0 \rangle$                     |  | 1371 | 0.00   |
| 25 | $\langle \Psi_{IJ}^{AB}  $ | $\hat{V}_N \Psi_0 \rangle$                               |  | 838  | -1.00  |
| 26 | $\langle \Psi_{IJ}^{AB}  $ | $\hat{V}_N \hat{T}_1 \hat{T}_1 \Psi_0 \rangle$           |  | 1869 | -1.00  |

|    |                            |                                                          |  |      |        |
|----|----------------------------|----------------------------------------------------------|--|------|--------|
| 27 | $\langle \Psi_{IJ}^{AB}  $ | $\hat{V}_N \hat{T}_2 \Psi_0 \rangle$                     |  | 2451 | 0.34   |
| 28 | $\langle \Psi_{IJ}^{AB}  $ | $\hat{F}_N \hat{T}_2 \Psi_0 \rangle$                     |  | 2236 | 0.00   |
| 29 | $\langle \Psi_{IJ}^{AB}  $ | $\hat{V}_N \hat{T}_1 \hat{T}_2 \Psi_0 \rangle$           |  | 2983 | -10.00 |
| 30 | $\langle \Psi_{IJ}^{AB}  $ | $\hat{V}_N \hat{T}_1 \hat{T}_1 \hat{T}_2 \Psi_0 \rangle$ |  | 3193 | -8.37  |
| 31 | $\langle \Psi_{IJ}^{AB}  $ | $\hat{F}_N \hat{T}_1 \hat{T}_2 \Psi_0 \rangle$           |  | 2477 | 1.63   |
| 32 | $\langle \Psi_{IJ}^{AB}  $ | $\hat{V}_N \hat{T}_1 \hat{T}_1 \Psi_0 \rangle$           |  | 2056 | -1.00  |
| 33 | $\langle \Psi_{IJ}^{AB}  $ | $\hat{V}_N \hat{T}_1 \hat{T}_1 \hat{T}_2 \Psi_0 \rangle$ |  | 2942 | 2.25   |
| 34 | $\langle \Psi_{IJ}^{AB}  $ | $\hat{V}_N \hat{T}_1 \hat{T}_1 \hat{T}_2 \Psi_0 \rangle$ |  | 2966 | -8.37  |
| 35 | $\langle \Psi_{IJ}^{AB}  $ | $\hat{V}_N \hat{T}_2 \hat{T}_2 \Psi_0 \rangle$           |  | 3238 | -7.71  |
| 36 | $\langle \Psi_{IJ}^{AB}  $ | $\hat{V}_N \hat{T}_1 \hat{T}_2 \Psi_0 \rangle$           |  | 2603 | 1.92   |
| 37 | $\langle \Psi_{IJ}^{AB}  $ | $\hat{V}_N \hat{T}_1 \hat{T}_2 \Psi_0 \rangle$           |  | 2935 | -10.00 |
| 38 | $\langle \Psi_{IJ}^{AB}  $ | $\hat{V}_N \hat{T}_2 \Psi_0 \rangle$                     |  | 2415 | 0.34   |
| 39 | $\langle \Psi_{IJ}^{AB}  $ | $\hat{V}_N \hat{T}_1 \hat{T}_1 \hat{T}_2 \Psi_0 \rangle$ |  | 3103 | -8.37  |
| 40 | $\langle \Psi_{IJ}^{AB}  $ | $\hat{V}_N \hat{T}_1 \hat{T}_1 \hat{T}_2 \Psi_0 \rangle$ |  | 3113 | 2.25   |
| 41 | $\langle \Psi_{IJ}^{AB}  $ | $\hat{V}_N \hat{T}_2 \hat{T}_2 \Psi_0 \rangle$           |  | 3456 | -21.00 |

|    |                            |                                                                    |                                                                                   |      |       |
|----|----------------------------|--------------------------------------------------------------------|-----------------------------------------------------------------------------------|------|-------|
| 42 | $\langle \Psi_{IJ}^{AB}  $ | $\hat{V}_N \hat{T}_2 \hat{T}_2 \Psi_0 \rangle$                     | 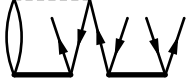 | 3239 | -7.71 |
| 43 | $\langle \Psi_{IJ}^{AB}  $ | $\hat{F}_N \hat{T}_2 \Psi_0 \rangle$                               | 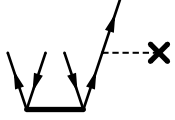 | 2252 | 0.00  |
| 44 | $\langle \Psi_{IJ}^{AB}  $ | $\hat{F}_N \hat{T}_1 \hat{T}_2 \Psi_0 \rangle$                     | 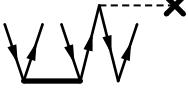 | 2527 | 1.63  |
| 45 | $\langle \Psi_{IJ}^{AB}  $ | $\hat{V}_N \hat{T}_1 \hat{T}_1 \hat{T}_1 \Psi_0 \rangle$           | 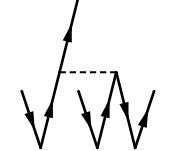 | 2351 | 1.92  |
| 46 | $\langle \Psi_{IJ}^{AB}  $ | $\hat{V}_N \hat{T}_1 \hat{T}_1 \hat{T}_1 \hat{T}_1 \Psi_0 \rangle$ | 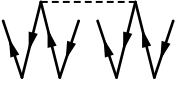 | 2376 | 2.25  |
| 47 | $\langle \Psi_{IJ}^{AB}  $ | $\hat{V}_N \hat{T}_2 \hat{T}_2 \Psi_0 \rangle$                     | 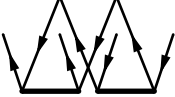 | 2710 | 8.45  |

## 2 Fixpoint iterative CCSD

Table 2: Collection of optimized Goldstone diagrams of the first and second iteration correlation energy, single and double projections in a fixpoint iterative post-non-canonical HF CCSD.

| Iteration 1 |                     |                                                                                     |
|-------------|---------------------|-------------------------------------------------------------------------------------|
| Energy      |                     |                                                                                     |
| Index       | Substitution        | Diagram                                                                             |
| 48          | $51 \rightarrow 0$  | 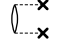   |
| 49          | $51 \rightarrow 1$  | 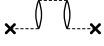   |
| 50          | $52 \rightarrow 2$  | 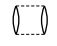   |
| Singles     |                     |                                                                                     |
| 51          | —                   | 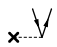   |
| Doubles     |                     |                                                                                     |
| 52          | —                   | 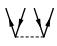   |
| Iteration 2 |                     |                                                                                     |
| Energy      |                     |                                                                                     |
| 53          | $203 \rightarrow 0$ | 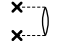   |
| 54          | $204 \rightarrow 0$ | 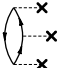 |
| 55          | $205 \rightarrow 0$ | 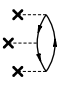 |
| 56          | $206 \rightarrow 0$ | 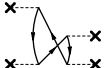 |
| 57          | $207 \rightarrow 0$ | 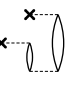 |
| 58          | $208 \rightarrow 0$ | 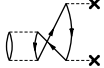 |
| 59          | $209 \rightarrow 0$ | 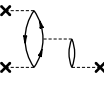 |
| 60          | $210 \rightarrow 0$ | 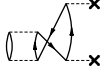 |
| 61          | $211 \rightarrow 0$ | 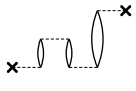 |
| 62          | $212 \rightarrow 0$ | 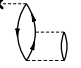 |
| 63          | $213 \rightarrow 0$ | 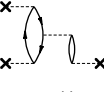 |
| 64          | $214 \rightarrow 0$ | 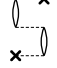 |

| Index | Substitution             | Diagram                                                                               |
|-------|--------------------------|---------------------------------------------------------------------------------------|
| 65    | $215 \rightarrow 0$      | 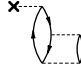   |
| 66    | $216 \rightarrow 0$      | 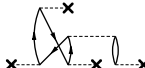   |
| 67    | $203, 203 \rightarrow 1$ | 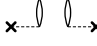   |
| 68    | $203, 204 \rightarrow 1$ | 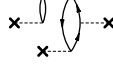   |
| 69    | $203, 205 \rightarrow 1$ | 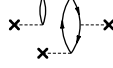   |
| 70    | $203, 206 \rightarrow 1$ | 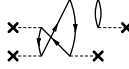   |
| 71    | $203, 207 \rightarrow 1$ | 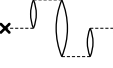   |
| 72    | $203, 208 \rightarrow 1$ | 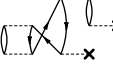   |
| 73    | $203, 209 \rightarrow 1$ | 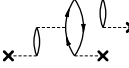  |
| 74    | $203, 210 \rightarrow 1$ | 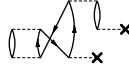 |
| 75    | $203, 211 \rightarrow 1$ | 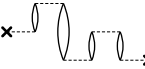 |
| 76    | $203, 212 \rightarrow 1$ | 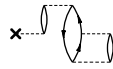 |
| 77    | $203, 213 \rightarrow 1$ | 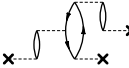 |
| 78    | $203, 214 \rightarrow 1$ | 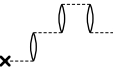 |
| 79    | $203, 215 \rightarrow 1$ | 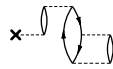 |
| 80    | $203, 216 \rightarrow 1$ | 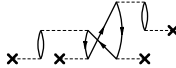 |
| 81    | $204, 204 \rightarrow 1$ | 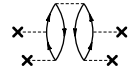 |
| 82    | $204, 205 \rightarrow 1$ | 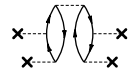 |
| 83    | $204, 206 \rightarrow 1$ | 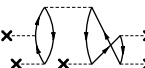 |
| 84    | $204, 207 \rightarrow 1$ | 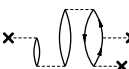 |

| Index | Substitution             | Diagram |
|-------|--------------------------|---------|
| 85    | 204, 208 $\rightarrow$ 1 |         |
| 86    | 204, 209 $\rightarrow$ 1 |         |
| 87    | 204, 210 $\rightarrow$ 1 |         |
| 88    | 204, 211 $\rightarrow$ 1 |         |
| 89    | 204, 212 $\rightarrow$ 1 |         |
| 90    | 204, 213 $\rightarrow$ 1 |         |
| 91    | 204, 214 $\rightarrow$ 1 |         |
| 92    | 204, 215 $\rightarrow$ 1 |         |
| 93    | 204, 216 $\rightarrow$ 1 |         |
| 94    | 205, 205 $\rightarrow$ 1 |         |
| 95    | 205, 206 $\rightarrow$ 1 |         |
| 96    | 205, 207 $\rightarrow$ 1 |         |
| 97    | 205, 208 $\rightarrow$ 1 |         |
| 98    | 205, 209 $\rightarrow$ 1 |         |
| 99    | 205, 210 $\rightarrow$ 1 |         |
| 100   | 205, 211 $\rightarrow$ 1 |         |
| 101   | 205, 212 $\rightarrow$ 1 |         |
| 102   | 205, 213 $\rightarrow$ 1 |         |
| 103   | 205, 214 $\rightarrow$ 1 |         |
| 104   | 205, 215 $\rightarrow$ 1 |         |
| 105   | 205, 216 $\rightarrow$ 1 |         |

| Index | Substitution             | Diagram |
|-------|--------------------------|---------|
| 106   | 206, 206 $\rightarrow$ 1 |         |
| 107   | 206, 207 $\rightarrow$ 1 |         |
| 108   | 206, 208 $\rightarrow$ 1 |         |
| 109   | 206, 209 $\rightarrow$ 1 |         |
| 110   | 206, 210 $\rightarrow$ 1 |         |
| 111   | 206, 211 $\rightarrow$ 1 |         |
| 112   | 206, 212 $\rightarrow$ 1 |         |
| 113   | 206, 213 $\rightarrow$ 1 |         |
| 114   | 206, 214 $\rightarrow$ 1 |         |
| 115   | 206, 215 $\rightarrow$ 1 |         |
| 116   | 206, 216 $\rightarrow$ 1 |         |
| 117   | 207, 207 $\rightarrow$ 1 |         |
| 118   | 207, 208 $\rightarrow$ 1 |         |
| 119   | 207, 209 $\rightarrow$ 1 |         |
| 120   | 207, 210 $\rightarrow$ 1 |         |
| 121   | 207, 211 $\rightarrow$ 1 |         |
| 122   | 207, 212 $\rightarrow$ 1 |         |
| 123   | 207, 213 $\rightarrow$ 1 |         |
| 124   | 207, 214 $\rightarrow$ 1 |         |
| 125   | 207, 215 $\rightarrow$ 1 |         |
| 126   | 207, 216 $\rightarrow$ 1 |         |

| Index | Substitution             | Diagram | Index | Substitution             | Diagram |
|-------|--------------------------|---------|-------|--------------------------|---------|
| 127   | 208, 208 $\rightarrow$ 1 |         | 148   | 210, 214 $\rightarrow$ 1 |         |
| 128   | 208, 209 $\rightarrow$ 1 |         | 149   | 210, 215 $\rightarrow$ 1 |         |
| 129   | 208, 210 $\rightarrow$ 1 |         | 150   | 210, 216 $\rightarrow$ 1 |         |
| 130   | 208, 211 $\rightarrow$ 1 |         | 151   | 211, 211 $\rightarrow$ 1 |         |
| 131   | 208, 212 $\rightarrow$ 1 |         | 152   | 211, 212 $\rightarrow$ 1 |         |
| 132   | 208, 213 $\rightarrow$ 1 |         | 153   | 211, 213 $\rightarrow$ 1 |         |
| 133   | 208, 214 $\rightarrow$ 1 |         | 154   | 211, 214 $\rightarrow$ 1 |         |
| 134   | 208, 215 $\rightarrow$ 1 |         | 155   | 211, 215 $\rightarrow$ 1 |         |
| 135   | 208, 216 $\rightarrow$ 1 |         | 156   | 211, 216 $\rightarrow$ 1 |         |
| 136   | 209, 209 $\rightarrow$ 1 |         | 157   | 212, 212 $\rightarrow$ 1 |         |
| 137   | 209, 210 $\rightarrow$ 1 |         | 158   | 212, 213 $\rightarrow$ 1 |         |
| 138   | 209, 211 $\rightarrow$ 1 |         | 159   | 212, 214 $\rightarrow$ 1 |         |
| 139   | 209, 212 $\rightarrow$ 1 |         | 160   | 212, 215 $\rightarrow$ 1 |         |
| 140   | 209, 213 $\rightarrow$ 1 |         | 161   | 212, 216 $\rightarrow$ 1 |         |
| 141   | 209, 214 $\rightarrow$ 1 |         | 162   | 213, 213 $\rightarrow$ 1 |         |
| 142   | 209, 215 $\rightarrow$ 1 |         | 163   | 213, 214 $\rightarrow$ 1 |         |
| 143   | 209, 216 $\rightarrow$ 1 |         | 164   | 213, 215 $\rightarrow$ 1 |         |
| 144   | 210, 210 $\rightarrow$ 1 |         | 165   | 213, 216 $\rightarrow$ 1 |         |
| 145   | 210, 211 $\rightarrow$ 1 |         | 166   | 214, 214 $\rightarrow$ 1 |         |
| 146   | 210, 212 $\rightarrow$ 1 |         | 167   | 214, 215 $\rightarrow$ 1 |         |
| 147   | 210, 213 $\rightarrow$ 1 |         | 168   | 214, 216 $\rightarrow$ 1 |         |

| Index | Substitution             | Diagram |
|-------|--------------------------|---------|
| 169   | $215, 215 \rightarrow 1$ |         |
| 170   | $215, 216 \rightarrow 1$ |         |
| 171   | $216, 216 \rightarrow 1$ |         |
| 172   | $217 \rightarrow 2$      |         |
| 173   | $218 \rightarrow 2$      |         |
| 174   | $219 \rightarrow 2$      |         |
| 175   | $220 \rightarrow 2$      |         |
| 176   | $221 \rightarrow 2$      |         |
| 177   | $222 \rightarrow 2$      |         |
| 178   | $223 \rightarrow 2$      |         |
| 179   | $224 \rightarrow 2$      |         |
| 180   | $225 \rightarrow 2$      |         |
| 181   | $226 \rightarrow 2$      |         |
| 182   | $227 \rightarrow 2$      |         |
| 183   | $228 \rightarrow 2$      |         |
| 184   | $229 \rightarrow 2$      |         |
| 185   | $230 \rightarrow 2$      |         |
| 186   | $231 \rightarrow 2$      |         |
| 187   | $232 \rightarrow 2$      |         |
| 188   | $233 \rightarrow 2$      |         |
| 189   | $234 \rightarrow 2$      |         |
| 190   | $235 \rightarrow 2$      |         |

| Index | Substitution        | Diagram |
|-------|---------------------|---------|
| 191   | $236 \rightarrow 2$ |         |
| 192   | $237 \rightarrow 2$ |         |
| 193   | $238 \rightarrow 2$ |         |
| 194   | $239 \rightarrow 2$ |         |
| 195   | $240 \rightarrow 2$ |         |
| 196   | $241 \rightarrow 2$ |         |
| 197   | $242 \rightarrow 2$ |         |
| 198   | $243 \rightarrow 2$ |         |
| 199   | $244 \rightarrow 2$ |         |
| 200   | $245 \rightarrow 2$ |         |
| 201   | $246 \rightarrow 2$ |         |
| 202   | $247 \rightarrow 2$ |         |

#### Singles

|     |                         |  |
|-----|-------------------------|--|
| 203 | —                       |  |
| 204 | $51 \rightarrow 4$      |  |
| 205 | $51 \rightarrow 5$      |  |
| 206 | $51 \rightarrow 6$      |  |
| 207 | $52 \rightarrow 7$      |  |
| 208 | $51, 52 \rightarrow 8$  |  |
| 209 | $51 \rightarrow 9$      |  |
| 210 | $51, 52 \rightarrow 10$ |  |
| 211 | $51, 52 \rightarrow 11$ |  |
| 212 | $52 \rightarrow 12$     |  |

| Index | Substitution        | Diagram |
|-------|---------------------|---------|
| 213   | $51 \rightarrow 13$ |         |
| 214   | $51 \rightarrow 14$ |         |
| 215   | $52 \rightarrow 15$ |         |
| 216   | $51 \rightarrow 16$ |         |

#### Doubles

|     |                         |  |
|-----|-------------------------|--|
| 217 | $51 \rightarrow 17$     |  |
| 218 | $51, 52 \rightarrow 18$ |  |
| 219 | $52 \rightarrow 19$     |  |
| 220 | $51, 52 \rightarrow 20$ |  |
| 221 | $51, 52 \rightarrow 21$ |  |
| 222 | $51 \rightarrow 22$     |  |
| 223 | $51 \rightarrow 23$     |  |
| 224 | $51 \rightarrow 24$     |  |
| 225 | —                       |  |
| 226 | $51 \rightarrow 26$     |  |
| 227 | $52 \rightarrow 27$     |  |
| 228 | $52 \rightarrow 28$     |  |
| 229 | $51, 52 \rightarrow 29$ |  |
| 230 | $51, 52 \rightarrow 30$ |  |
| 231 | $51, 52 \rightarrow 31$ |  |
| 232 | $51 \rightarrow 32$     |  |
| 233 | $51, 52 \rightarrow 33$ |  |
| 234 | $51, 52 \rightarrow 34$ |  |

| Index | Substitution            | Diagram |
|-------|-------------------------|---------|
| 235   | $52 \rightarrow 35$     |         |
| 236   | $51, 52 \rightarrow 36$ |         |
| 237   | $51, 52 \rightarrow 37$ |         |
| 238   | $52 \rightarrow 38$     |         |
| 239   | $51, 52 \rightarrow 39$ |         |
| 240   | $51, 52 \rightarrow 40$ |         |
| 241   | $52 \rightarrow 41$     |         |
| 242   | $52 \rightarrow 42$     |         |
| 243   | $52 \rightarrow 43$     |         |
| 244   | $51, 52 \rightarrow 44$ |         |
| 245   | $51 \rightarrow 45$     |         |
| 246   | $51 \rightarrow 46$     |         |
| 247   | $52 \rightarrow 47$     |         |
